# Supplementary material for: Miniaturizing transmon qubits using van der Waals materials
Source: arXiv:2109.02824 source file (2022-05-14)
Supplement: Supplementary file 1 [file Supplementary.tex]

longbibliography, superscriptaddress]{revtex4-1}
%\documentclass[12pt, showpacs, longbibliography, superscriptaddress]{revtex4-1}
%\usepackage{fullpage}
\usepackage{graphicx}% Include figure files
\usepackage{lipsum}
\usepackage{dcolumn}% Align table columns on decimal point
\usepackage{bm}% bold math
\usepackage{color}
\usepackage{amsmath, amsthm, amssymb}
\usepackage[modulo]{lineno}%[switch]{lineno} 
\usepackage[usenames,dvipsnames]{xcolor}
\usepackage[normalem]{ulem}
%\usepackage{ulem}
%\usepackage{setspace}
\newcommand{\ba}{\begin{eqnarray}}
\newcommand{\ea}{\end{eqnarray}}

\usepackage[colorlinks=true, urlcolor=violet, linkcolor=blue, citecolor=red, hyperindex=true, linktocpage=true]{hyperref}

\usepackage{float}
\floatstyle{boxed}
\begin{document}
\title{Supplementary Information}

%\subsection{vdW qubit parameters}





\end{document}
